# Supplementary material for: SoK: Pragmatic Assessment of Machine Learning for Network Intrusion Detection
Source: arXiv:2305.00550 source file (2023-04-30)
Supplement: Supplementary file 1 [file _extra.tex]

\begin{table*}[!htbp]
  \centering
  \caption{\dataset{CTU13} Multi-classification results.}
        \resizebox{2.0\columnwidth}{!}{
        \begin{tabular}{c|c ? cc|cc? cc|cc? cc|cc? cc|cc}
             \multicolumn{2}{c?}{Labelling} & \multicolumn{4}{c?}{100 (N=1000)} & \multicolumn{4}{c?}{20\% (N=100)} &  \multicolumn{4}{c?}{50\% (N=100)} &  \multicolumn{4}{c}{100\% (N=100)} \\ \hline
             \multicolumn{2}{c?}{Features} &
             \multicolumn{2}{c|}{Extended} & \multicolumn{2}{c?}{Essential} & \multicolumn{2}{c|}{Extended} & \multicolumn{2}{c?}{Essential} & \multicolumn{2}{c|}{Extended} & \multicolumn{2}{c?}{Essential} & \multicolumn{2}{c|}{Extended} & \multicolumn{2}{c}{Essential}  \\ \hline
            Alg. & Arch. & 
            iid & iid? & iid & iid? & 
            iid & iid? & iid & iid? & 
            iid & iid? & iid & iid? & 
            iid & iid? & iid & iid? \\
             \toprule
             
             \multirow{2}{*}{\rotatebox{90}{\parbox{40pt}\centering\textbf{RF}}}
             & MD & \\
             & B+MD & \\ 
             \midrule
             \multirow{2}{*}{\rotatebox{90}{\parbox{40pt}\centering\textbf{DT}}}
             & MD & \\
             & B+MD & \\ 
             \midrule
             \multirow{2}{*}{\rotatebox{90}{\parbox{40pt}\centering\textbf{LR}}}
             & MD & \\
             & B+MD & \\ 
             \midrule
             \multirow{2}{*}{\rotatebox{90}{\parbox{40pt}\centering\textbf{HGB}}}
             & MD & \\
             & B+MD & \\ 
             \bottomrule
             \end{tabular} 
             }
             \label{tab:ctu_multi}
\end{table*}

\begin{table*}[!htbp]
  \centering
  \caption{\dataset{CTU13} Training Times.}
        \resizebox{0.7\columnwidth}{!}{
        \begin{tabular}{c|c ? cc? cc? cc? cc}
             \multicolumn{2}{c?}{Labelling} & \multicolumn{2}{c?}{100 (N=1000)} & \multicolumn{2}{c?}{20\% (N=100)} &  \multicolumn{2}{c?}{50\% (N=100)} &  \multicolumn{2}{c}{100\% (N=100)} \\ \hline
              \hline
            Alg. & Arch. & 
            P1 & P2 &
            P1 & P2 &
            P1 & P2 &
            P1 & P2  \\
             \toprule
             
             \multirow{4}{*}{\rotatebox{90}{\parbox{40pt}\centering\textbf{RF (100\%)}}}
             & BD & \\
             & MD & \\ 
             & ED & \\ 
             & ED-s & \\ 
             \midrule
             
             \multirow{4}{*}{\rotatebox{90}{\parbox{40pt}\centering\textbf{DT (2.6\%)}}}
             & BD & \\
             & MD & \\ 
             & ED & \\ 
             & ED-s & \\ 
             \midrule
             
             \multirow{4}{*}{\rotatebox{90}{\parbox{40pt}\centering\textbf{LR (100\%)}}}
             & BD & \\
             & MD & \\ 
             & ED & \\ 
             & ED-s & \\ 
             \midrule
             
             \multirow{4}{*}{\rotatebox{90}{\parbox{40pt}\centering\textbf{HGB (100\%)}}}
             & BD & \\
             & MD & \\ 
             & ED & \\ 
             & ED-s & \\

             \bottomrule
             \end{tabular} 
             }
             \label{tab:ctu_training}
\end{table*}

\begin{table*}[!htbp]
  \centering
  \caption{\dataset{CTU13} Inference Time.}
        \resizebox{1.3\columnwidth}{!}{
        \begin{tabular}{c|c ? ccc? ccc? ccc? ccc}
             \multicolumn{2}{c?}{Labelling} & \multicolumn{3}{c?}{100 (N=1000)} & \multicolumn{3}{c?}{20\% (N=100)} &  \multicolumn{3}{c?}{50\% (N=100)} &  \multicolumn{3}{c}{100\% (N=100)} \\ \hline
              \hline
            Alg. & Arch. & 
            P1 & P2 & P3 &
            P1 & P2 & P3 &
            P1 & P2 & P3 &
            P1 & P2 & P3 \\
             \toprule
             
             \multirow{4}{*}{\rotatebox{90}{\parbox{40pt}\centering\textbf{RF (100\%)}}}
             & BD & \\
             & MD & \\ 
             & ED & \\ 
             & ED-s & \\ 
             \midrule
             
             \multirow{4}{*}{\rotatebox{90}{\parbox{40pt}\centering\textbf{DT (2.6\%)}}}
             & BD & \\
             & MD & \\ 
             & ED & \\ 
             & ED-s & \\ 
             \midrule
             
             \multirow{4}{*}{\rotatebox{90}{\parbox{40pt}\centering\textbf{LR (100\%)}}}
             & BD & \\
             & MD & \\ 
             & ED & \\ 
             & ED-s & \\ 
             \midrule
             
             \multirow{4}{*}{\rotatebox{90}{\parbox{40pt}\centering\textbf{HGB (100\%)}}}
             & BD & \\
             & MD & \\ 
             & ED & \\ 
             & ED-s & \\ 
              
             \bottomrule
             \end{tabular} 
             }
             \label{tab:ctu_inference}
\end{table*}
