# Supplementary material for: SoK: Pragmatic Assessment of Machine Learning for Network Intrusion Detection
Source: arXiv:2305.00550 source file (2023-04-30)
Supplement: Supplementary file 3 [file _multi.tex]

\begin{table*}[!htbp]
  \centering
  \caption{\dataset{temp} Multi-classification results.}
        \resizebox{2.0\columnwidth}{!}{
        \begin{tabular}{c|c ? cc|cc? cc|cc? cc|cc? cc|cc}
             \multicolumn{2}{c?}{Available Data} & \multicolumn{4}{c?}{Limited (100 per class)} & \multicolumn{4}{c?}{Scarce (20\% of \scbb{D})} &  \multicolumn{4}{c?}{Moderate (40\% of \scbb{D})} &  \multicolumn{4}{c}{Abundant (80\% of \scbb{D})} \\ \hline
             \multicolumn{2}{c?}{Features} &
             \multicolumn{2}{c|}{Static [N=1000]} & \multicolumn{2}{c?}{Temporal [N=1]} & \multicolumn{2}{c|}{Static [N=1000]} & \multicolumn{2}{c?}{Temporal [N=1]} & \multicolumn{2}{c|}{Static [N=1000]} & \multicolumn{2}{c?}{Temporal [N=1]} & \multicolumn{2}{c|}{Static [N=1000]} & \multicolumn{2}{c?}{Temporal [N=1]}  \\ \hline
            Alg. & Arch. & 
            Complete & Essential & Complete & Essential & 
            Complete & Essential & Complete & Essential & 
            Complete & Essential & Complete & Essential & 
            Complete & Essential & Complete & Essential \\
             \toprule
             
             \multirow{2}{*}{\rotatebox{90}{\parbox{40pt}\centering\textbf{RF}}}
             & MD & \\
             & B+MD & \\ 
             \midrule
             \multirow{2}{*}{\rotatebox{90}{\parbox{40pt}\centering\textbf{DT}}}
             & MD & \\
             & B+MD & \\ 
             \midrule
             \multirow{2}{*}{\rotatebox{90}{\parbox{40pt}\centering\textbf{LR}}}
             & MD & \\
             & B+MD & \\ 
             \midrule
             \multirow{2}{*}{\rotatebox{90}{\parbox{40pt}\centering\textbf{HGB}}}
             & MD & \\
             & B+MD & \\ 
             \bottomrule
             \end{tabular} 
             }
             \label{tab:_multi}
\end{table*}
