# Supplementary material for: SoK: Pragmatic Assessment of Machine Learning for Network Intrusion Detection
Source: arXiv:2305.00550 source file (2023-04-30)
Supplement: Supplementary file 4 [file _open.tex]

\begin{table*}
  \centering
  \caption{\dataset{tempdata13} Results in open world scenarios (against both adversarial and unknown attacks).}

    \begin{subtable}[htbp]{1.95\columnwidth}
        \resizebox{1.0\columnwidth}{!}{
        \begin{tabular}{c|c ? cc|cc? cc|cc? cc|cc? cc|cc}
\multicolumn{2}{c?}{Available Data} & \multicolumn{4}{c?}{Limited (100 per class) [N=1000]} & \multicolumn{4}{c?}{Scarce (20\% of \scbb{D}) [N=100]} &  \multicolumn{4}{c?}{Moderate (40\% of \scbb{D}) [N=100]} &  \multicolumn{4}{c}{Abundant (80\% of \scbb{D}) [N=100]} \\ \hline
             \multicolumn{2}{c?}{Scenario} &
             \multicolumn{2}{c|}{Adversarial Attacks} & \multicolumn{2}{c?}{Unknown Attacks} & \multicolumn{2}{c|}{Adversarial Attacks} & \multicolumn{2}{c?}{Unknown Attacks} & \multicolumn{2}{c|}{Adversarial Attacks} & \multicolumn{2}{c?}{Unknown Attacks} & \multicolumn{2}{c|}{Adversarial Attacks} & \multicolumn{2}{c?}{Unknown Attacks}  \\ \hline
            Alg. & Design & 
            \footnotesize{$tpr$} \tiny{(org)} & \footnotesize{$tpr$} \tiny{(adv)} & \footnotesize{$fpr$} & \footnotesize{$tpr$} & \footnotesize{$tpr$} \tiny{(org)} & \footnotesize{$tpr$} \tiny{(adv)} & \footnotesize{$fpr$} & \footnotesize{$tpr$} & \footnotesize{$tpr$} \tiny{(org)} & \footnotesize{$tpr$} \tiny{(adv)} & \footnotesize{$fpr$} & \footnotesize{$tpr$} & \footnotesize{$tpr$} \tiny{(org)} & \footnotesize{$tpr$} \tiny{(adv)} & \footnotesize{$fpr$} & \footnotesize{$tpr$} \\
             \toprule
             
             \multirow{5}{*}{\rotatebox{90}{\parbox{40pt}\centering\textbf{RF}}} 
             & BD & \\
             & MD & \\
             & ED-f & \\ 
             & ED-v & \\
             & ED-s & \\
             & ED-o & \\
             
            \midrule
            \multirow{5}{*}{\rotatebox{90}{\parbox{40pt}\centering\textbf{DT}}} 
             & BD & \\
             & MD & \\
             & ED-f & \\ 
             & ED-v & \\
             & ED-s & \\
             & ED-o & \\
             \midrule
            \multirow{5}{*}{\rotatebox{90}{\parbox{40pt}\centering\textbf{LR}}} 
             & BD & \\
             & MD & \\
             & ED-f & \\ 
             & ED-v & \\
             & ED-s & \\
             & ED-o & \\
             \midrule
            \multirow{5}{*}{\rotatebox{90}{\parbox{40pt}\centering\textbf{HGB}}} 
             & BD & \\
             & MD & \\
             & ED-f & \\ 
             & ED-v & \\
             & ED-s & \\
             & ED-o & \\
            
            \bottomrule
        \end{tabular}
        }
                
        \caption{\dataset{tempdata13} Results in the absence of tempporal dependency.} 
    \label{tab:tempdata_open_static}
    \end{subtable}

    \begin{subtable}[htbp]{1.4\columnwidth}
        \resizebox{1.0\columnwidth}{!}{
        \begin{tabular}{c|c ? cc|cc? cc|cc? cc|cc? cc|cc}
\multicolumn{2}{c?}{Available Data} & \multicolumn{4}{c?}{Limited (100 per class) [N=1]} & \multicolumn{4}{c?}{Scarce (20\% of \scbb{D}) [N=1]} &  \multicolumn{4}{c?}{Moderate (40\% of \scbb{D}) [N=1]} &  \multicolumn{4}{c}{Abundant (80\% of \scbb{D}) [N=1]} \\ \hline
             \multicolumn{2}{c?}{Scenario} &
             \multicolumn{2}{c|}{Adversarial Attacks} & \multicolumn{2}{c?}{Unknown Attacks} & \multicolumn{2}{c|}{Adversarial Attacks} & \multicolumn{2}{c?}{Unknown Attacks} & \multicolumn{2}{c|}{Adversarial Attacks} & \multicolumn{2}{c?}{Unknown Attacks} & \multicolumn{2}{c|}{Adversarial Attacks} & \multicolumn{2}{c?}{Unknown Attacks}  \\ \hline
            Alg. & Design & 
            \footnotesize{$tpr$} \tiny{(org)} & \footnotesize{$tpr$} \tiny{(adv)} & \footnotesize{$fpr$} & \footnotesize{$tpr$} & \footnotesize{$tpr$} \tiny{(org)} & \footnotesize{$tpr$} \tiny{(adv)} & \footnotesize{$fpr$} & \footnotesize{$tpr$} & \footnotesize{$tpr$} \tiny{(org)} & \footnotesize{$tpr$} \tiny{(adv)} & \footnotesize{$fpr$} & \footnotesize{$tpr$} & \footnotesize{$tpr$} \tiny{(org)} & \footnotesize{$tpr$} \tiny{(adv)} & \footnotesize{$fpr$} & \footnotesize{$tpr$} \\
             \toprule
             
             \multirow{5}{*}{\rotatebox{90}{\parbox{40pt}\centering\textbf{RF}}} 
                          & BD & \\
             & MD & \\
             & ED-f & \\ 
             & ED-v & \\
             & ED-s & \\
             & ED-o & \\
             
            \midrule
            \multirow{5}{*}{\rotatebox{90}{\parbox{40pt}\centering\textbf{DT}}} 
             & BD & \\
             & MD & \\
             & ED-f & \\ 
             & ED-v & \\
             & ED-s & \\
             & ED-o & \\
             \midrule
            \multirow{5}{*}{\rotatebox{90}{\parbox{40pt}\centering\textbf{LR}}} 
             & BD & \\
             & MD & \\
             & ED-f & \\ 
             & ED-v & \\
             & ED-s & \\
             & ED-o & \\
             \midrule
            \multirow{5}{*}{\rotatebox{90}{\parbox{40pt}\centering\textbf{HGB}}} 
             & BD & \\
             & MD & \\
             & ED-f & \\ 
             & ED-v & \\
             & ED-s & \\
             & ED-o & \\
            
            \bottomrule
        \end{tabular}
        }
                
        \caption{\dataset{tempdata13} Results that assume `temporal' dependency between samples.} 
    \label{tab:tempdata_open_temporal}
    \end{subtable}

    \label{tab:tempdata_open}
\end{table*}
